# Supplementary material for: Measuring the Robustness of NLP Models to Domain Shifts
Source: arXiv:2306.00168 source file (2024-04-20)
Supplement: Supplementary file 1 [file 8a.old_results_appendix.tex]

\ZG{Start with a high level overview of your findings, then the goal of the rest of the section is to support these findings and convince the reader that they are true. i.e. separate the finding from the details of how you came to this finding. You can see example in page 6 here https://arxiv.org/pdf/2206.14796.pdf. In general - imagine you give an elevator speech on your findings and cannot dive into details.}
% \subsection{DR Scenarios}
% \label{sub:results_dr_scenarios}

\medskip\noindent\textbf{R.1 Question:} How do fine-tuned and few-shot learning models differ in the DR challenge?
% \smallskip\noindent\textbf{Visualizations:} 

Figure~\ref{fig:scenarios} compares the best-performing fine-tuned model to several few-shot learning models.
% \smallskip\noindent\textbf{Results:}
(1) For all tasks, fine-tuned models outperform few-shot learning models, achieving higher average in-domain and average cross-domain performance;
(2) Few-shot learning models seem more robust to domain shift, as their drops are consistently lower than those of fine-tuned models.
(3) The average drop in the SA task of the few-shot learning models with an instruction-tuning phase (GPT-JT, ChatGPT and GPT-4) is positive. However, the worst drops are not, and in the magnitude of the other models. \ZG{he sentence is not clrear and the takeaway from it is not clear.}
(4) In the NLI task, in-domain demonstrations seem to have a negative effect on the performance of GPT-4, since the average cross-domain performance is higher than the average in-domain performance.\ZG{Why do we bother with this detail? Does it help you to deliver your takeaway?}


\ZG{The takeaway is that few-shot models are more robust, right?}

\smallskip\noindent\textbf{Limitations:} See R.2 and R.3 Limitations. \ZG{I would avoid these and just have one limitations section at the end of the paper.}



\medskip\noindent\textbf{R.2 Question:} What DR scenarios are common in each task (see \S\ref{sub:scenarios})? 

% \smallskip\noindent\textbf{Visualizations:} 
Figure~\ref{fig:scenarios} presents the distribution of each scenario for each task.
% \smallskip\noindent\textbf{Results:}
(1) The Classic DR challenge, which occurs when both $\sd$ and $\td$ are positive, is the most common scenario. For fine-tuning classification tasks, as well as the AS task, the Classic scenario dominates in more than 70\% of the cases; \ZG{What can we learn from that?}
(2) Notice that the four scenarios are prevalent in all of the few-shot learning tasks, and in that case, we may say that the effect of the domain shift is weak. It is also the case in the fine-tuning QA and QG tasks, which share the same partition of examples into domains and therefore might behave similarly;
(3) The Unobserved DR challenge scenario (positive $\td$ but negative $\sd$) is common, occurring in 7 out of 8 fune tuning tasks (ranging between 11\% in SA to 40\% in TG), and in all few-shot learning tasks occurring in noticeable proportions. This observation is important since many of the past works looked only at $\sd$, and our study suggests that a DR challenge may exist (in terms of positive $\td$) even if participants do not observe a performance degradation;
(4) The Observed DR challenge (positive $\sd$ but negative $\td$), while not as common as the Unobserved scenario, still occurs in 4 out of the 8 fine-tuning tasks and in all few-shot learning tasks. These results highlight the importance of our proposed additional perspective (i.e., the $\td$) on performance degradation. 

\ZG{The finding here is that TD is indeed important.}

\smallskip\noindent\textbf{Limitations:} This analysis includes all the participating models that may lead to a broader and more general picture of the challenge. In addition, it neither discusses the magnitude of the performance drops nor the scores. In what comes next, we  present scores and drops of specific models. \ZG{I would avoid these and just have one limitations section at the end of the paper.}

% \subsection{Fine-tuning}
% \label{sub:results_finetuning}

\medskip\noindent\textbf{R.3 Question:} What is the relationship between the fine-tuned model size and the DR challenge?

% \smallskip\noindent\textbf{Visualizations:} 
Figures~\ref{fig:scenarios} and \ref{fig:scenarios} which present the performance and the drops of fine-tuned models, for classification and generation tasks, respectively. We present the average in-domain and cross-domain performance, and the average worst $\sd$ and $\td$. 
% \smallskip\noindent\textbf{Results:}
(1) For all tasks and models, the average in-domain performance is higher than the average cross-domain performance,except for the QA and QG tasks, where the difference between the two is minor (Notice that the QA and QG tasks share the same partition of examples into domains);
\ZG{Waht can we learn from this?}
(2) The magnitude of the average drop differs between the tasks, for example, the Average Drop in the AE task, which is around 50 F1 points, is much larger than in the QA tasks, which is around one F1 point;
\ZG{Waht can we learn from this?}
(3) Larger models of the same architecture family improve the average in-domain and the average cross-domain performance scores; 
(4) Regarding the performance gap, the general trend is that larger models improve \ZG{reduce?} performance drops;
(5) For all tasks and models, the Average Worst $\sd$ is larger than the Average Worst $\td$. We will discuss this finding later when answering R.5.\ZG{So discuss it in R.5.}

\ZG{Summarize what is the key takeaway? Larger models are more robust? Isn't this expected? Are there any other takeaways?}

\ZG{The figures are too overloaded, this comes in line with my comments about too many metrics. You don't even discuss all the details and metrics here. e.g. why do you need the top and the bottom row to make you point? Maybe in this case the vizualization part is not so strong and you can arrange the scores in a table, maybe with heat map for values.} 

\smallskip\noindent\textbf{Limitations:} We did not fine-tune models with more than one billion parameters due to computational reasons.\ZG{I would avoid these and just have one limitations section at the end of the paper.}

\medskip\noindent\textbf{R.3 Question:} What is the relationship between the few-shot model size and the DR challenge?

% \smallskip\noindent\textbf{Visualizations:} 
Figure~\ref{fig:scenarios} presents the average performance scores of several few-shot learning models and the average drops as a function of the size. 
% \smallskip\noindent\textbf{Results:}
% (1) For all tasks and models, the average in-domain performance is higher than the cross-domain performance;
% (2) Similar to fine-tuning, increasing the model size improves both the average in-domain and cross-domain performance of few-shot learning models, as illustrated by the OPT-family model curves;
% (3) Larger models do not improve the performance drop and the effect of the size on the DR challenge is not clear.
As illustrated by the OPT-family model curves -- while increasing the model size improves both the average in-domain and cross-domain (absolute) performance, it does not improve the performance drop. We conclude that the magnitude of the DR challenge is not clear in the few-shot scenario. This can be attributed to the fact that few-shot models usually exposed to many domains during pre-training and that the few shot exemplars do not adapt the model to the relevant topical domain, but only provide task-related guidance. 
% , although a U pattern can be observed;

\smallskip\noindent\textbf{Limitations:} 
Few-shot learning models typically require several to dozens of demonstrations as input, especially when the texts are short. However, due to the system's maximum token length of 2048 and the long nature of our texts, we used a maximum of 4 demonstrations in our analysis. Surprisingly, when we attempted the NLI task involving short texts, we found that increasing the number of demonstrations up to 12 led to a continued decrease in performance. Moreover, it is important to note that few-shot learning models can be sensitive to the demonstrations or instructions provided \citep{instruction_sensitivity, prompt_sensitivity}, and different prompts may yield different results. Additionally, for generation tasks, the performance of GPT-family models may be difficult to evaluate automatically. Upon manual inspection of the outputs generated by these models, we found them comparable or even superior to the reference texts.\ZG{I would avoid these and just have one limitations section at the end of the paper.}

% \subsection{Fine-tuning vs. Few-shot Learning}
% \label{sub:results_finetuning}


% \subsection{DR Characterization}
% \label{sub:results_characterizing}

\medskip\noindent\textbf{R.4 Question:} Given the DR has two aspects, $\sd$ and $\td$, what is their relationship with $\st$? 

% \smallskip\noindent\textbf{Visualizations:} 
Table~\ref{tab:characterizing} presents statistics on $\sd$ and $\td$, including their std deviations, the Worst drops, and the correlations of $\st$ with $\sss$ and $\ttt$.
% \smallskip\noindent\textbf{Results:}
(1) For every task and for both fine-tuning and few-shot learning models, the variance of $\sd$ is larger than the variance of $\td$ (with and exception of the NLI task for few-shot learning). 
(2) For almost every task, the Worst and the Average Worst $\sd$ is larger than  Sometimes, the average worst $\sd$ is two to three times bigger (e.g., QG and TG). An exception is the SA task, where the worst $\td$ is bigger. This result indicates that the observed degradation attributed to domain shift in the majority of DR works might not tell the whole story. \ZG{I thought that we already convinced the reader that this is the case and I cannot see why these STD and variance numbers are needed.} In \S\ref{sec:discussion}, we discuss the impact of this finding on DR research;\ZG{I really don't like this "promo" style, this requires the reader to keep a memory cache of information. Discuss the finding and its inpact in once place.}
(3) The Worst $\sd$ and Worst $\td$ suggest that in every task and model, there is a substantial performance drop. Accordingly, the challenging shifts indicate that the DR challenge is still relevant. Moreover, the large differences between the Average Drop and the Worst $\sd$ and $\td$ drops suggest that synthetic domain shifts, like challenge sets that typically focus on hard shifts, do not represent the average robustness of NLP models truthfully;
(4) The correlation between $\st$ and $\ttt$ is much stronger than the correlation with $\sss$, and for most fine-tuning tasks, it is above 0.8. This result can explain why the variance and the Worst drops of the $\sd$ are larger than the ones of the $\td$. Accordingly, we find the $\ttt$ to approximate the $\st$ better, and consequently, the $\td$ approximates better the Average Drop than the $\sd$.
(5) Nevertheless, when the DR problem is severe, the $\ttt$ is not informative for the $\st$. For example, the AE task, which has the highest degradation in performance (more than 20 F1 points) has the weakest correlations. In contrast, the strongest correlations are observed for the QA and the QG tasks, demonstrating the lowest performance drops.

\medskip\noindent\textbf{R.6 Question:} What is the relationship between the number of few-shot demonstrations and the DR challenge?

\smallskip\noindent\textbf{Visualizations:} Figure~\ref{fig:scenarios} presents the average performance scores and average drops as a function of the number of demonstrations. 

\smallskip\noindent\textbf{Results:}
(1) Compared to zero-shot learning, few-shot learning improves both the average in-domain and cross-domain performance, except for the OPT-6.7b model in the SA task, which exhibits lower average cross-domain performance for one and two demonstrations;
(2) For all tasks except NLI, the average cross-domain performance is consistently lower than the average in-domain performance, regardless of the number of demonstrations. This indicates on a DR challenge in few-shot learning, although it is weak;
(3) The domain of the demonstrations impacts the performance. To the best of our knowledge, this is the first study to show this;
(4) While increasing the number of demonstrations can improve both the in-domain and cross-domain performance, it does not necessarily minimize the gap between the two (i.e., the drop). The NLI task is an exception, where increasing the number of demonstrations actually harms performance.

\smallskip\noindent\textbf{Limitations:} See R.3 Limitations.
